# Supplementary material for: Silicon-Vacancy Spin Qubit in Diamond: A Quantum Memory Exceeding 10 ms with Single-Shot State Readout
Source: arXiv:1708.08852 ancillary file (2017-12-04)
Supplement: Supplementary file 1 [file SiVspinSI.pdf]

# Supplemental Material for
# The silicon-vacancy spin qubit in diamond: quantum memory exceeding ten milliseconds and single-shot state readout

D. D. Sukachev,[1,*] A. Sipahigil,[1,*] C. T. Nguyen,[1,*] M. K. Bhaskar,[1] R. E. Evans,[1] F. Jelezko,[2] and M. D. Lukin[1,†]

[1]*Department of Physics, Harvard University, 17 Oxford Street, Cambridge, Massachusetts 02138, USA**
[2]*Institute for Quantum Optics, Ulm University and Center for Integrated Quantum Science and Technology, Albert-Einstein-Allee 11, 89081 Ulm, Germany*

## I. DILUTION REFRIGERATOR SETUP

We use a BlueFors BF-LD250 cryogen-free dilution refrigerator (DR) modified to obtain free-space optical access (see Fig. S1). For optical excitation and collection, we use a home-built confocal microscope. We excite SiVs resonantly with $\sim$ 737-nm light and use occasional off-resonant 520-nm pulses to reset the SiV charge state [1, 2]. We combine these beams on a dichroic mirror (DM). SiV fluorescence in the phonon side-band (PSB) is collected using a 90:10 non-polarizing beam-splitter cube (BSC), coupled to a multi-mode (MM) fiber, and sent to a single-photon detector (APD). For spectral filtering, we use a short-pass filter (SP) in the excitation arm and band-pass filters (BP) in the collection arm. The optics used to deliver light into and to collect light from the DR are mounted on a breadboard (Thorlabs PBG12102) on top of the frame supporting the DR. This allows for DR venting and sample exchange without realignment of the optics.

A collimated laser beam enters at the top of the DR through a vacuum viewport (1) using the central line-of-sight port. The optical beam is focused on the diamond sample (12) by a low-temperature compatible objective (4). To reduce the heat load due to black-body radiation at the mixing chamber plate (MXC), 10-mm apertures (2) are installed at each stage inside the DR. In this configuration, the base temperature at the MXC is 20 mK. We do not use any cold windows along the optical path inside the DR.

A 6-1-1 T cryogen-free superconducting vector magnet (14) is mounted below the MXC and thermally linked to the 4 K plate of the DR. The diamond sample (12) is soldered with indium to a fixed copper sample holder (13) and placed inside the magnet bore on a science plate (11). We operate this magnet in a persistent mode to reduce $SiV^-$ spin dephasing due to fluctuations of applied magnetic fields.

A vented cryo-compatible objective (4) is mounted on 3-axis piezo steppers (8, 10, 5) and 3-axis piezo scanners (6) via L-brackets (3). X-Y steppers (8, 10) are mounted on the science plate (11) which is connected to the MXC via two copper rods (not shown). The diamond sample holder (13) and the science plate (11) are thermally anchored to the MXC via oxygen-free copper braids (Copper Braid Products). Thermalization plates (7,9) and the objective L-bracket (3) are thermally anchored to the science plate via copper braids (11).

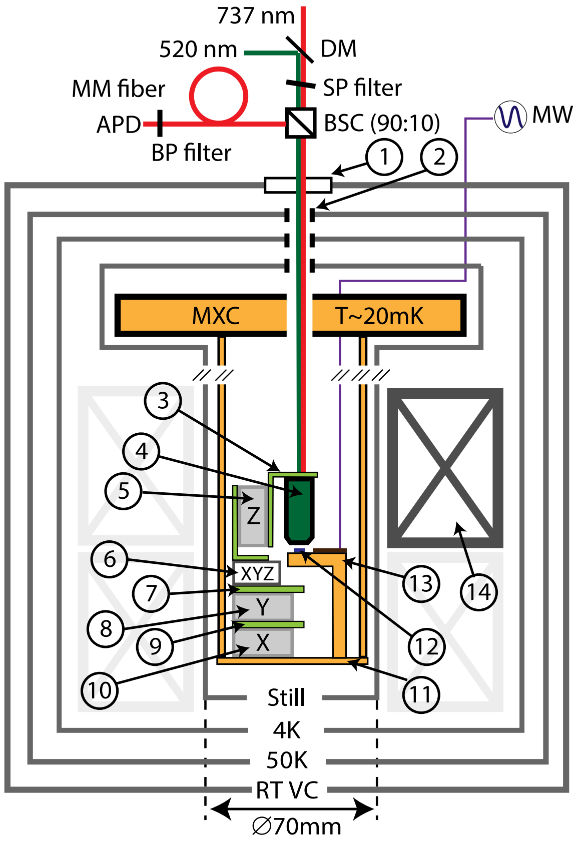


FIG. S1. Schematic of a dilution refrigerator with free-space optical access. MXC: Mixing chamber plate; Still: Still plate; 4K: 4K plate; 50K: 50K plate; RT VC: Outer vacuum can; SP: 758-nm short-pass filter (Semrock FF01-758/SP-25), tilted by a small angle to tune the cut-off frequency; BP: Band-pass filters (Semrock FF01-775/46-25 and FF01-785/62-25); MM: 25 um-core MM fiber; DM: dicroic mirror (Semrock Di03-R561-t1-25x36); APD: Single-photon counting module; BSC: Non-polarizing beam-splitter cube with T:R = 90:10; 1: vacuum viewport; 2: 10-mm apertures at 50 K, 4 K and Still plates of the DR; 3: Objective L-bracket 4: Low-temperature, vacuum compatible objective (Attocube LT-APO-VISIR) with NA = 0.82; 5: Attocube stepper (ANPx311) which moves the objective vertically; 6: Three-axis Attocube scanner (ANSxyz100); 7,9: Thermalization plates, each braided to (11); 8,10: 2 Attocube steppers ANPx311 which position the sample laterally; 11: A science plate positioned inside a vector magnet (14) and thermally anchored to the MXC; 12: Diamond sample; 13: Sample holder; 14: Cryogen-Free MAxes 6-1-1 T superconducting vector magnet with persistent switches (American Magnetics Inc.).

* These authors contributed equally
† lukin@physics.harvard.edu

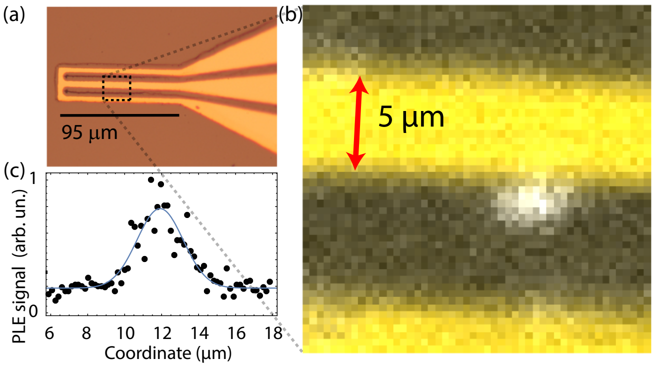


FIG. S2. (a) Room temperature micrograph of the shorted gold coplanar waveguides fabricated on the diamond surface. (b) Low temperature false color reflection image of the diamond surface (black) and the coplanar waveguide (gold), overlaid with the PLE image of an $SiV^-$ (white). (c) Cross-section of the $SiV^-$ PLE image. The optical resolution is 3 $\mu$m.

Microwave (MW) pulses are delivered to the diamond sample via coaxial lines (semi-rigid 2.19mm SCuNi-CuNi lines between room temperature and 4K, superconducting 0.86mm NbTi-NbTi lines between 4K and MXC) which are thermalized at each stage. A temperature sensor (Lake Shore Cryotronics, RX-102B-CB) is placed on the sample holder (13) and measures a sample temperature of $\leq$ 100 mK in the absence of microwave driving.

We fabricate shorted coplanar waveguides on the diamond surface to efficiently deliver MW pulses (Fig. S2). To fabricate these striplines, we first deposit 50 nm of Ti and 600 nm of Au onto the diamond surface using thermal evaporation. Next, a photolithography mask is patterned on the surface, and the unmasked Au and Ti are selectively etched away using Transene Gold Etchant Type TFA diluted 2:1 with water for 2 min, then 5.6% HF by weight (49% HF diluted 9:1 with water) for 30 s.

We adjust focus with the stepper (5) and use other two steppers (8, 10) for coarse positioning. We take confocal images of the diamond sample by moving the objective using piezo scanners (6). Optical resolution of the microscope is $\approx 3\,\mu$m (Fig. S2) and is limited by residual mechanical noise from a pulse tube and the collection pinhole diameter (25 $\mu$m) set by the MM fiber.

## II. 3-LEVEL SATURATION MEASUREMENTS

In Fig. 1(d) of the Main Text, we compare the PSB counts during resonant excitation of transitions C and D (PLE spectroscopy). Laser driving can affect steady-state population of the UB or the LB via optically pumping to the opposite branch [Fig. S3(a)]. This effect is minimized when laser power is below the three-level saturation intensity set by the decay rate of the excited state ($\gamma_0$) and the phonon relaxation rates ($\gamma_\uparrow$ and $\gamma_\downarrow$). By solving master equations for the corresponding 3-level system, we find that at temperatures $T < 1$ K, for which the thermal population of phonon modes at the frequency $\Delta_{\rm GS}$ is $n(T, \Delta_{\rm GS}) \to 0$, the saturation intensity is $\propto \gamma_\downarrow/\gamma_0$. The downward phonon relaxation rate is $\gamma_\downarrow \propto (n(T, \Delta_{\rm GS}) + 1)$ [3] and does not depend on T in this regime. Thus, saturation intensity is also constant for $T < 1$ K.

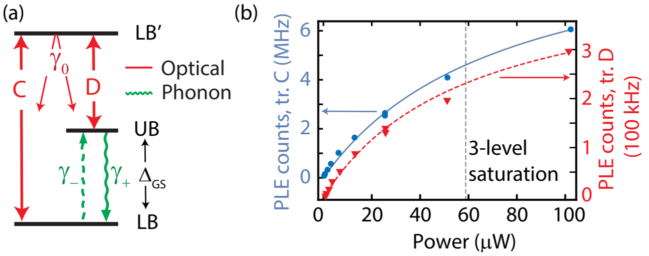


FIG. S3. Three-level saturation in PLE measurements. (a) Relaxation rates in the three-level system formed by the LB and the UB of the $SiV^-$ ground state and the first excited state (LB′). $\gamma_0$ is the total decay rate from the excited state; $\gamma_+(\gamma_-)$ is the upward (downward) phonon relaxation rate. (b) Saturation measurement of the PLE intensity. Blue data is displaced vertically for clarity. Vertical dashed line represents the laser power at 3-level saturation. Power is measured before entering the DR.

In Fig. S3(b), we measure PLE counts for transitions C and D at different laser powers at the fixed $T = 0.75$ K. For both transitions, saturation corresponds to a laser power of $\sim 60\,\mu$W. Since at $T = 0.75$ K, $n < 0.1$, saturation intensity does not change at lower $T$ and can only increase at higher temperatures due to faster phonon relaxation.

In Fig. 1(d), we use a laser power of 0.5 $\mu$W and thus work deep below 3-level saturation for the whole temperature range. In this case, the ratio of PLE counts is proportional to the ratio of the thermal populations of the LB and the UB of the $SiV^-$ ground state as stated in the Main Text.

## III. MAGNETIC FIELD ALIGNMENT FOR SINGLE-SHOT SPIN READOUT

The cyclicity of the spin-conserving transitions depends on the angle between the SiV symmetry axis and applied magnetic field $\vec{B}$ [4]. In this section, we describe our procedure to align the magnetic field to the SiV symmetry axis with

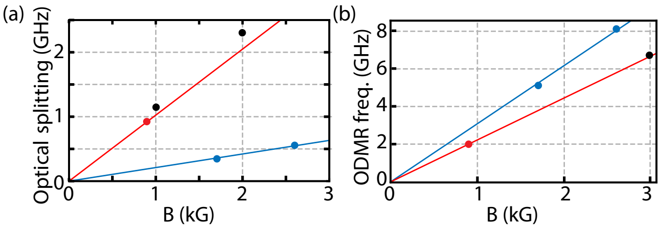


FIG. S4. (a) Splitting of spin-selective transitions in a magnetic field and (b) ODMR frequency. Red data: Orthogonal field for $SiV^-$ with $\Delta_{\rm GS} = 75$ GHz in Sample 12; Blue: the same $SiV^-$ in an aligned field. Black: SiV with $\Delta_{\rm GS} = 85$ GHz in Sample 13 in an orthogonal field. Solid lines are linear fits.

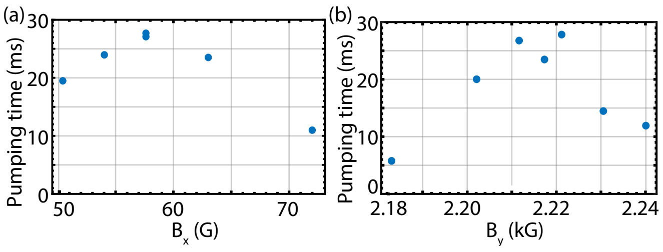


FIG. S5. Magnetic field alignment (a) Optical pumping times at different $B_x$ at $\{B_y = 2.2\,\text{kG}, B_z = 1.5\,\text{kG}\}$. (b) Optical pumping times at different $B_y$ at $\{B_x = 63\,\text{G}, B_z = 1.5\,\text{kG}\}$

$0.1^\circ$ precision. The SiV symmetry axis can be pointed along four possible $\langle 111\rangle$ orientations in the diamond lattice. Based on the Hamiltonian in Ref. [5], the Zeeman splittings of the ground states and excited states depend on both the orientation of the magnetic field and the amount of strain in the crystal. For strained emitters with $50\,\text{GHz} < \Delta_{\text{GS}} < 100\,\text{GHz}$, off-axis magnetic fields lead to a larger Zeeman splitting in the ground states compared with the excited states. Magnetic fields along the symmetry axis, however, result in a comparable Zeeman splitting in ground and excited states. As shown in Fig. S4(a), this leads to a larger frequency splitting between spin-conserving transitions for misaligned fields. We use this approach to determine the orientation group of an SiV center.

For a given $\text{SiV}^-$, we apply a magnetic field along all 4 possible SiV orientations $\langle 111\rangle$. Based on the discussion above, the smallest optical splitting corresponds to the magnetic field pointed along the SiV axis. Experimentally, this procedure gives a pointing error of few degrees.

Finally, we fine tune the orientation of the magnetic field by probing SiV spin dynamics. Fig. S5 shows measured optical spin pumping times at different field orientations. These measurements indicate that the spin dynamics are very sensitive to the magnetic field orientation and a precision of $\sim 0.1^\circ$ degrees is required to scatter photons for 30 ms without a spin flip.

## IV. SCATTERING RATES AND COLLECTION EFFICIENCY

For measurements in Fig. 3(e) in the Main Text, power of the readout laser is set at a 3-level saturation (see sec. II). This maximizes the number of scattered photons and minimizes off-resonant excitation of the other spin-conserving transition. In this case, the lifetime of the metastable UB $\tau = \gamma_\downarrow^{-1}$ limits the photon absorption rate to $R \sim 1/\tau$. For an unstrained emitter ($\Delta_{\text{GS}} \approx 45\,\text{GHz}$), $\tau \sim 200\,\text{ns}$ at 100 mK [3]. Since the phonon emission probability is proportional to $(\Delta_{\text{GS}})^3$, the absorption rate for a strained $\text{SiV}^-$ is $R \sim \frac{1}{200\,\text{ns}} \cdot \left(\frac{\Delta_{\text{GS}}[\text{GHz}]}{45\,\text{GHz}}\right)^3$. During a 20 ms readout window, the $\text{SiV}^-$ in Fig. 3(e) should absorb $\sim 2 \times 10^5$ photons. In the same readout window we detect $\sim 10$ photons. Thus, the overall system efficiency is $\sim 2 \times 10^{-4}$. This assumes a $\sim 10\%$ quantum efficiency for the $\text{SiV}^-$ [1] optical transition and a $\sim 30\%$ fraction of the PSB (Debye-Waller Factor) in the total emission spectrum.

We can also estimate the collection efficiency in a different way. At 3-level saturation, the steady-state PLE count rate is also limited by $1/\tau \approx 5 \times 10^6\,\text{Hz}$. In our experiment, the typical steady-state PLE count rate are $10^3\,\text{Hz}$. This gives $\sim 2 \times 10^{-4}$ for the overall system efficiency which agrees with the previous estimate.

## V. OPTICAL SPIN INITIALIZATION AND READOUT

To initialize the $\text{SiV}^-$ qubit, in state $|\uparrow\rangle$ for example, we drive the spin-resolved transition $|\downarrow\rangle \rightarrow |\downarrow'\rangle$. Optical pumping [Fig. 2(a)] eventually brings the qubit into state $|\uparrow\rangle$. For higher initialization fidelity, the initialization laser pulse was several times longer than the characteristic time $t_p$ for optical pumping [Fig. 2(d)].

We optically readout the qubit states by driving the corresponding spin-conserving transition. For better readout signal-to-noise, we keep the duration of the readout pulse to less than the optical pumping time $t_p$. Intensities of both initialization and readout pulses were at 3-level saturation (see sec. II).

## VI. SPIN LIFETIME MEASUREMENT

We measure a lower bound for the spin lifetime ($T_1$) of the $\text{SiV}^-$ spin qubit in a magnetic field of 1.1 kG aligned along the $\text{SiV}^-$ axis within a few degrees. Pulse sequence for the $T_1$ measurement is illustrated in Fig. S6. First, a 3-ms long laser pulse at frequency $f_{\downarrow\downarrow'}$ initializes the qubit in state $|\uparrow\rangle$. Next, a readout laser at frequency $f_{\uparrow\uparrow'}$ probes the population in state $|\uparrow\rangle$ at time $t_0$ and pumps the qubit into state $|\downarrow\rangle$. After a delay $\tau$, we probe the population in state $|\uparrow\rangle$ again. The remaining spin polarization depends on the $T_1$ time. The corresponding pulse sequence is shown in Fig. S6(b).

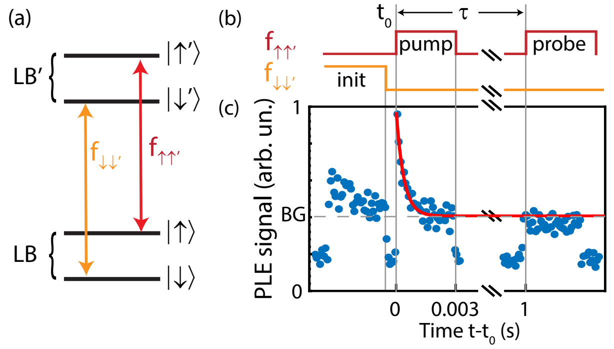


FIG. S6. $\text{SiV}^-$ spin $T_1$ measurement. (a) Simplified level structure of the $\text{SiV}^-$. $f_{\downarrow\downarrow'}$ and $f_{\uparrow\uparrow'}$ are frequencies of spin-conserving transitions. (b) Pulse sequence for spin $T_1$ measurement (see text) (c) Time-resolved PLE signal for a sequence in b). BG denotes a level of background fluorescence.

We measure the absence of any fluorescence signal above the background level (BG) after a delay of $\tau = 1\,\text{s}$ [Fig. S6(c)]. This indicates an almost perfect spin polarization after 1 s and means that the SiV$^-$ spin $T_1$ is much greater than 1 s.

## VII. MICROWAVE DRIVING

We use the SiV states $|\uparrow\rangle$ and $|\downarrow\rangle$ as a spin qubit. In a small aligned magnetic field $B$ ($\mu_\text{B} B \ll h\lambda_\text{SO}$), these states are of the form [5]

$$|\uparrow\rangle = |\uparrow\rangle_\text{spin} \otimes \left( |e_-\rangle + \frac{1-\sqrt{1+\xi^2}}{\xi} |e_+\rangle \right)$$

$$|\downarrow\rangle = |\downarrow\rangle_\text{spin} \otimes \left( |e_+\rangle + \frac{1-\sqrt{1+\xi^2}}{\xi} |e_-\rangle \right)$$

$$\xi = \frac{\alpha}{\lambda_\text{SO}},$$

where $\alpha$ is an off-diagonal ($E_g$) strain [6], $\lambda_\text{SO} \approx 46\,\text{GHz}$ is the spin-orbit coupling in the ground manifold of the SiV $\left(\Delta_\text{GS} = \sqrt{\alpha^2 + \lambda_\text{SO}^2}\right)$; $|\uparrow\rangle_\text{spin}, |\downarrow\rangle_\text{spin}$ are spin states; and $|e_+\rangle, |e_-\rangle$ are orthogonal electronic orbital states.

To coherently manipulate the SiV spin qubit, we drive the transition $|\uparrow\rangle \to |\downarrow\rangle$ with resonant MW pulses. The Rabi frequency is $\Omega_\text{MW} \sim \sqrt{P_\text{MW}} \cdot \frac{1-\sqrt{1+\xi^2}}{\xi}$, where $P_\text{MW}$ is the MW power. We verify a square-root dependence of $\Omega_\text{MW}$ on the MW power in Fig. S7.

In the low strain regime ($\alpha \ll \lambda_\text{SO}$), the qubit magnetic dipole transition $|\downarrow\rangle \to |\uparrow\rangle$ is only weakly allowed. This makes a coherent control of the spin with the MW driving difficult due to heating of the sample via ohmic losses in the gold stripline.

In this work, we use SiV centers with $\Delta_\text{GS} \approx 80\,\text{GHz}$. A corresponding moderate crystal strain of $\alpha \approx 1.5\lambda_\text{SO}$ allows the qubit transition and reduces the necessary amount of MW power. This facilitates maintaining a steady-state sample temperature of $\sim 100\,\text{mK}$.

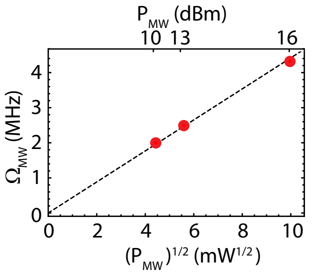


FIG. S7. Frequency of MW Rabi oscillations ($\Omega_\text{MW}$) at different MW powers ($P_\text{MW}$) delivered to the dilution fridge. The power at the sample is reduced by an estimated $\sim 5\,\text{dB}$ due to losses in the coaxial lines. The dashed line is a linear fit. Data are taken at $f_{\downarrow\uparrow} = 6.6\,\text{GHz}$

## VIII. $T_2^*$ LIMITING PROCESSES AND PULSE ERRORS

The measurements in Fig. 3 of the Main Text demonstrate that $T_2^*$ scales approximately inversely with the static magnetic field in the isotopically purified sample (Sample 12). In this section, we discuss a microscopic mechanism that can lead to the observed $(T_2^*)^{-1} \propto g\mu_B B$ dependence. As discussed in Sec. VII and Ref. [5], the wavefunction of the spin qubit consists of both an electronic orbital and a spin degree of freedom that each contribute to the electronic Landé g-factor.

The electronic orbitals $|e_-\rangle$ and $|e_+\rangle$ can be mixed via strain and large electric fields. The mixing mechanism via strain is described in Sec. VII. While electric fields cannot mix the two orbitals $|e_-\rangle$ and $|e_+\rangle$ that have the same parity to first order, second-order processes (mediated by the excited states of the opposite parity) can result in a mixing between the two orbitals. The presence of such electric or strain field fluctuations can therefore lead to fluctuation of the orbital wavefunctions and a corresponding change in the g-factor of the qubit states. This can cause a spin dephasing at a rate proportional to an applied magnetic field $B$.

The resulting $T_2^*$ also limits the single qubit gate fidelities. We operate with MW Rabi frequencies $\Omega_\text{MW}$ in the range from 1 to 10 MHz. In this case, MW $\pi$-time of $\sim 100\,\text{ns}$ is comparable with $T_2^*$ resulting in imperfect MW $\pi$-pulses with errors at the percent level. For CPMG sequences involving 32 rephasing $\pi$-pulses [Fig. 4(b)], this results in a reduction of the state fidelity to $\sim 70\%$ level. In our experiments, stronger MW driving (corresponding to larger $\Omega_\text{MW}$) causes heating of the sample due to Ohmic losses in a gold coplanar waveguide which destroys spin coherence [Fig. 4(d)]. By using low-loss superconducting coplanar waveguide [7] for MW delivering, larger $\Omega_\text{MW}$ can be achieved without additional heat load.

## IX. COUPLING TO NUCLEAR SPINS

The effect of a $^{13}$C nuclear spin on a spin-echo signal depends on the ratio of the external magnetic field and the magnetic field produced by an SiV$^-$ at the nuclear site (Knight shift) [8]. In a large external magnetic field of 3 kG, this Knight shift is negligible and we do not observe any effect

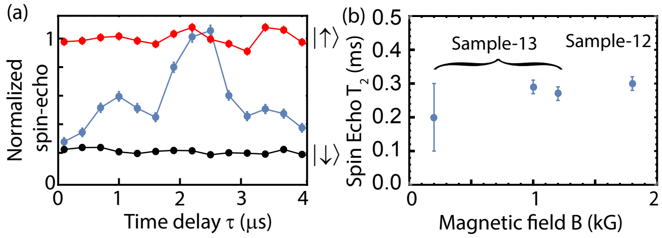


FIG. S8. Spin echo at different magnetic fields. (a) Spin-echo curves for $\tau < 4\,\mu\text{s}$. Blue data: Spin echo at $B = 0.2\,\text{kG}$; Black data: Spin echo at $B = 3\,\text{kG}$; Red data: Spin echo at $B = 3\,\text{kG}$, the second $\pi/2$ pulse is replaced by $3\pi/2$. (b) Spin-echo ($T_2$) times at different magnetic fields.

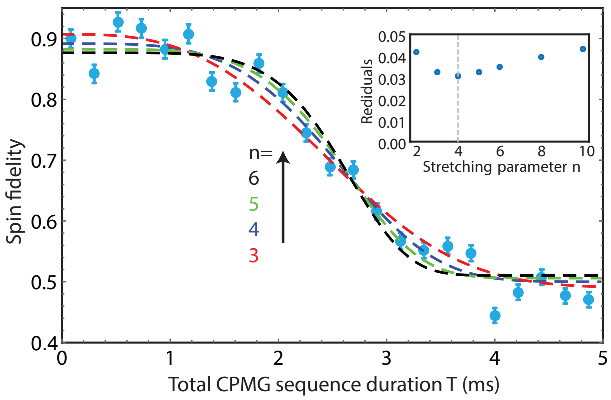


FIG. S9. Experimental CPMG curve with $N = 8$ (blue points) fitted by stretched exponentials with $n = 3, 4, 5, 6$. Inset: fit residuals for stretched exponentials with $n = 2, 3, 4, 5, 6, 8, 10$.

of nuclear spins in the spin-echo measurements [black data in Fig. S8(a)]. We repeated this measurement with a spin-echo sequence modified such that the second $\pi/2$ pulse was replaced by a $3\pi/2$ pulse (red data). This allows us to normalize the readout signal. The mean value of the spin-echo (modified spin-echo) signal at $\tau \ll T_2$ corresponds to find the SiV$^-$ spin in state $|\downarrow\rangle$ ($|\uparrow\rangle$).

In contrast, repeating these measurements in a low magnetic field of 0.2 kG yields high-visibility oscillations of the SiV$^-$ spin coherence [blue data in Fig. S8(a)] suggesting a coherent coupling to several $^{13}$C nuclear spins in Sample 13.

Coherent coupling to nuclear spins does not affect the $T_2$ time as measured by the spin-echo envelope [Fig. S8(b)]. We observe the same $T_2$ times for Sample 13 in magnetic fields from 0.2 kG to 1 kG and for Sample 12 in a 2 kG magnetic field. This suggests that coupling to nuclear spins is not the main factor which limits the SiV$^-$ spin $T_2$ time.

## X. SPIN COHERENCE ANALYSIS

Various systematic effects—such as calibration errors of the readout levels, coherent dynamics with the $^{13}$C nuclear spin bath, or different MW gate fidelities for different experimental runs (due to e.g. uncalibrated slow drifts in the system)—may affect fidelities of CPMG sequences [Fig. 4(b)]. Since we have not studied these systematic effects in detail, we present the data with minimal data processing: For each curve in Fig. 4(b), the measured background is subtracted from the signal and the result is normalized such that the steady state value is equal to 1/2, corresponding to an equal mixture between the qubit levels; no additional rescaling is implemented.

The observed scaling of the coherence time $T_2$ with number $N$ of rephasing pulses [Fig. 4(c)] is close to linear: $T_2 \propto N^\beta$, where $\beta = 1.02 \pm 0.05$. This scaling contradicts dephasing due to a pure Lorentzian noise power spectrum which gives $T_2 \sim N^{2/3}$ [9, 10].

Different noise bath models can produce similar $T_2$ scaling but lead to different shapes of the CPMG curves. Fig. S9 shows the CPMG8 curve [from Fig. 4(b)] fitted with different stretched exponentials $\exp\left[-\left(T/T_0\right)^n\right]$. To fit the experimental data in Fig. 4(b), we use a stretched exponential with $n = 4$ since is gives the smallest fit residuals (Fig. S9, inset). Using the present data it is not possible to distinguish between different noise models as we can't directly deconvolve the noise power spectrum [10, 11].

In Fig. 3(f), we show the dependance of the $T_2^*$ time on the magnetic field amplitude which indicates additional noise in the system (see sec. VIII). In contrast, we do not observe any dependence of the $T_2$ time on magnetic field [Fig. S8(c)]. This suggests a bimodal noise power spectrum: a slow-frequency component limits the $T_2^*$ time while a high-frequency component determines the $T_2$ time. For example, a double-Gaussian noise power spectrum:

$$S(\omega) = A \times \exp\left[-\left(\omega/\omega_0\right)^2\right] + B \times \exp\left[-\left(\omega/\omega_1\right)^2\right], \quad (1)$$

where $A \approx 10^6\,\mathrm{s}^{-1}$, $\omega_0 \approx 1.8 \cdot 10^3\,\mathrm{s}^{-1}$, $B \approx 10^9\,\mathrm{s}^{-1}$, and $\omega_1 \approx 50\,\mathrm{s}^{-1}$, provides a good agreement with the observed $T_2$ scaling [Fig. S10(a)] and the correct order-of-magnitude for $T_2^* \approx 10\,\mu$s. In this case, the calculated CPMG8 curve is close to a stretched exponential with $n = 4$ [Fig. S10(b)]. The same result can be obtained using a double-Lorentzian noise power spectrum with hard frequency cutoffs [12].

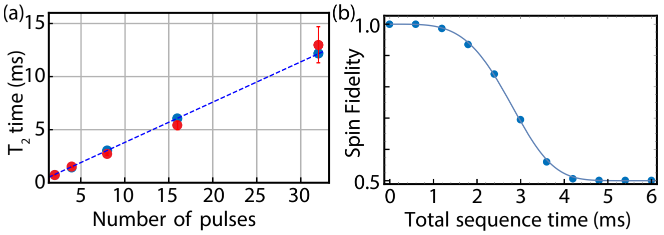


FIG. S10. Double-Gaussian noise power spectrum. (a) Calculated $T_2$ times for CPMG sequences (blue points) and measured $T_2$ times (red points). Dashed line is a linear fit. (b) Calculated CPMG8 curve (dots) fitted by a strecthed exponential with $n = 4$ (solid line).


[1] A. Sipahigil, R. E. Evans, D. D. Sukachev, M. J. Burek, J. Borregaard, M. K. Bhaskar, C. T. Nguyen, J. L. Pacheco, H. A. Atikian, C. Meuwly, R. M. Camacho, F. Jelezko, E. Bielejec, H. Park, M. Lončar, and M. D. Lukin, Science **354**, 847 (2016).

[2] R. E. Evans, A. Sipahigil, D. D. Sukachev, A. S. Zibrov, and M. D. Lukin, Physical Review Applied **5**, 044010 (2016).

[3] K. D. Jahnke, A. Sipahigil, J. M. Binder, M. W. Doherty, M. Metsch, L. J. Rogers, N. B. Manson, M. D. Lukin, and F. Jelezko, New Journal of Physics **17**, 043011 (2015).

[4] L. J. Rogers, K. D. Jahnke, T. Teraji, L. Marseglia, C. Müller, B. Naydenov, H. Schauffert, C. Kranz, J. Isoya, L. P. McGuinness, and F. Jelezko, Nature communications **5**, 4739 (2014).

[5] C. Hepp, T. Müller, V. Waselowski, J. N. Becker, B. Pingault, H. Sternschulte, D. Steinmüller-Nethl, A. Gali, J. R. Maze, M. Atatüre, and C. Becher, Physical Review Letters **112**, 036405 (2014).

[6] Y.-I. Sohn, S. Meesala, B. Pingault, H. A. Atikian, J. Holzgrafe, M. Gundogan, C. Stavrakas, M. J. Stanley, A. Sipahigil, J. Choi, *et al.*, arXiv preprint 1706.03881 (2017).

[7] A. J. Sigillito, H. Malissa, A. M. Tyryshkin, H. Riemann, N. V. Abrosimov, P. Becker, H.-J. Pohl, M. L. Thewalt, K. M. Itoh, J. J. Morton, *et al.*, Applied Physics Letters **104**, 222407 (2014).

[8] L. Childress, M. V. Gurudev Dutt, J. M. Taylor, A. S. Zibrov, F. Jelezko, J. Wrachtrup, P. R. Hemmer, and M. D. Lukin, Science **314** (2006).

[9] N. Bar-Gill, L. Pham, A. Jarmola, D. Budker, and R. Walsworth, Nature Communications **4**, 1743 (2013).

[10] J. Medford, Ł. Cywiński, C. Barthel, C. M. Marcus, M. P. Hanson, and A. C. Gossard, Physical Review Letters **108**, 086802 (2012).

[11] N. Bar-Gill, L. Pham, C. Belthangady, D. Le Sage, P. Cappellaro, J. Maze, M. Lukin, A. Yacoby, and R. Walsworth, Nature communications **3**, 858 (2012).

[12] M. J. Biercuk and H. Bluhm, Phys. Rev. B **83**, 235316 (2011).
